# Supplementary material for: A Deep Neural Networks ensemble workflow from hyperparameter search to inference leveraging GPU clusters
Source: arXiv:2208.14046 source file (2022-08-30)
Supplement: Supplementary file 1 [file appendix_1_kaggle.tex]

\clearpage
\section{Ensemble awards in past public image recognition challenges}
\label{sec:kaggle}

\vspace{-0.1cm}
URL : \href{https://ndres.me/kaggle-past-solutions/}{https://ndres.me/kaggle-past-solutions}
\vspace{-0.1cm}

\begin{itemize}
\setlength\itemsep{-0.3em}
\item \textbf{\textbf{Name:}} \textbf{Understanding Clouds from Satellite Images}
\item \textbf{Description:} Can you classify cloud structures from satellites?
\item \textbf{Participation:} 1538 teams
\item \textbf{Prize:} \$10K
\item \textbf{Dead line:} 2019-11-19
\item \textbf{1st place} – Use averaging predictions of 3 segmentations models; averaging 9 segmentations models
\item \textbf{3rd place} – Use majority vote of 4 segmentations models
\item \textbf{4th place} – Averaging of 10 models
\item \textbf{5th place} – Weighted averaging of 3 segmentations models
\end{itemize}

\vspace{-0.1cm}

\begin{itemize}
\setlength\itemsep{-0.25em}
\item \textbf{\textbf{Name:}} \textbf{RSNA Intracranial Hemorrhage Detection}
\item \textbf{Description:} Identify acute intracranial hemorrhage and its subtypes
\item \textbf{Participation:} 1345 teams
\item \textbf{Prize:}  \$25K
\item \textbf{Dead line:} 2019-10-28\
\item \textbf{2st place} – 15 bagging LSTMs (3 bootstraps) 
\item \textbf{3rd place} - Use weighted averaging predictions of 17 models
\item \textbf{5th place} – Stacking of 9 segmentation models
\end{itemize}

\vspace{-0.1cm}

\begin{itemize}
\setlength\itemsep{-0.25em}
\item \textbf{Name:} \textbf{Lyft 3D Object Detection for Autonomous Vehicles}
\item \textbf{Description:} Can you advance the state of the art in 3D object detection?
\item \textbf{Participation:} 547 teams
\item \textbf{Prize:} \$25K
\item \textbf{Dead line:} 2019-11-3 
\item \textbf{3rd place} – 3 faster-rcnn models with Soft NMS
\end{itemize}

\vspace{-0.1cm}

\begin{itemize}
\setlength\itemsep{-0.25em}
\item \textbf{Name:} \textbf{Severstal Steel Defect Detection}
\item \textbf{Description:} Can you detect and classify defects in steel?
\item \textbf{Participation:} 2431 teams
\item \textbf{Prize:} \$120K
\item \textbf{Dead line:} 2019-10-18
\item \textbf{1st place} – Ensemble of 4 classifications (which one ?);  Ensemble of 9 segmentations(which one ?)
\item \textbf{4th place}  – Ensemble of 9 segmentations (which one ?)
\end{itemize}

\vspace{-0.1cm}

\begin{itemize}
\setlength\itemsep{-0.25em}
\item \textbf{Name:} \textbf{Kuzushiji Recognition}
\item \textbf{Description:} Opening the door to a thousand years of Japanese culture
\item \textbf{Participation:} 293 teams
\item \textbf{Prize:} \$15K
\item \textbf{Dead line:} 2019-10-15
\item \textbf{1st place} – Ensemble of 2 R-CNN
\item \textbf{2nd place} – 1 Faster-RCNN, Stacking with an ensemble of XGBoost and LightGBM averaging
\item \textbf{3rd place} – Hard voting of 5 models; NMS with 2 models
\end{itemize}

\vspace{-0.1cm}

\begin{itemize}
\setlength\itemsep{-0.25em}
\item \textbf{Name:} \textbf{The 3rd YouTube-8M Video Understanding Challenge}
\item \textbf{Description:} Temporal localization of topics within video
\item \textbf{Participation:} 283 teams
\item \textbf{Prize:} \$25K
\item \textbf{Dead line:} 2019-10-04
\item \textbf{1st place} – 17 averaging models + smooth out predictions 
\item \textbf{2nd place} – 7 models weighted averaging, weights fixed manually 
\item \textbf{3rd place} – Stacking of 12 models
\end{itemize}

\vspace{-0.1cm}

\begin{itemize}
\setlength\itemsep{-0.25em}
\item \textbf{Name:} \textbf{APTOS 2019 Blindness Detection}
\item \textbf{Description:} Detect diabetic retinopathy to stop blindness before it's too late
\item \textbf{Participation:} 2931 teams
\item \textbf{Prize:} \$50K
\item \textbf{1st place} – Ensemble of 8 models with stacking
\item \textbf{4th place} – Averaging of 3 models
\end{itemize}
