# Supplementary material for: A Deep Neural Networks ensemble workflow from hyperparameter search to inference leveraging GPU clusters
Source: arXiv:2208.14046 source file (2022-08-30)
Supplement: Supplementary file 2 [file appendix_3_automl.tex]

\clearpage
\section*{AutoML workflows comparison}
\label{sec:appautoml}

Here a summary of AutoML tools list \ref{tab:appautoml}.  Some of them have automatic pre-processing hyperparameters to control pre-processing but auto-keras. We do not mention pre-processing in this paper to focus on the efficiency. In the Image case, H2O driverless AI have resolution as hyperparameter. We use 5 hyperparameters to control the data augmentation process. 

H2O Driverless IA is a commercial tool as far we search, we do not find the hyperparameter optimization algorithm used.  Due to the difficulty to find relevant information we do not mention other commercial AutoML tools.

\begin{table}[hbt!]
\small
\setlength\tabcolsep{4pt}
%\centering
\begin{tabularx}{\textwidth}{llllllll}
\toprule
Name              & Backend        & Image ?  & Optimization                                                                    & Ens. sel. criteria                                                                 & Ens. sel. strategy                                                          & Ensemble combiner                                                                       \\
\midrule
Auto WEKA \cite{autoweka}         & WEKA           & No                                & SMAC                                                                            & 5 models                               & Ad hoc                                                                          & Voting or Stacking                                                                   \\[0.4cm]
Auto Sklearn  \cite{autosklearn}     & sklearn   & No                                 & \begin{tabular}[c]{@{}l@{}}SMAC \\ Distributed with Dask \end{tabular}                                                                            & Nb. models user given                & Forward greedy                                                                      & Averaging                                                                               \\[0.4cm]
TPOT       \cite{tpot}        & sklearn   & No                                 & \begin{tabular}[c]{@{}l@{}}Genetic Programming \\ Distributed with Dask \end{tabular}                                                           & -                                                                                       & -                                                                           & -                                                                                       \\[0.4cm]
H2O AutoML  \footnote{\url{https://docs.h2o.ai/}}        & H2O            & No                              & \begin{tabular}[c]{@{}l@{}}Random Search \\ Distributed (Spark)\end{tabular}    & 1 model for each model family        & The best of each family                                                         & Stacking                                                                                \\[0.4cm]
H2O Driverless AI \cite{h2odriverless}  & H2O            & Yes                              & \begin{tabular}[c]{@{}l@{}}??? \\ Distributed with Spark\end{tabular}               & Nb. models user given                  & Ad hoc                                                                           & Averaging                                                                               \\[0.4cm]
Auto Keras  \cite{autokeras}      & Keras          & Yes                              & Bayesian with NN Kernel                                                         & -                                                                                       & -                                                                           & -                                                                                       \\[0.4cm]
\textbf{Ours}     & \textbf{Keras} & \textbf{Yes}               & \textbf{\begin{tabular}[c]{@{}l@{}}Hyperband or SMAC\\ Distributed with Ray \end{tabular}} & \textbf{\begin{tabular}[c]{@{}l@{}}Computing budget user given\end{tabular}} & \textbf{\begin{tabular}[c]{@{}l@{}}SMOBF greedy\\Distributed with Ray \end{tabular}} & \textbf{\begin{tabular}[c]{@{}l@{}}Averaging\\Distributed with Ray \end{tabular}} \\
\bottomrule
\end{tabularx}
\caption{Comparison of AutoML workflows. The mention "-" means the workflow does not use ensemble. The mention "???" means the information is not present in the documentation.}
\label{tab:appautoml}
\end{table}
