# Supplementary material for: A Deep Neural Networks ensemble workflow from hyperparameter search to inference leveraging GPU clusters
Source: arXiv:2208.14046 source file (2022-08-30)
Supplement: Supplementary file 4 [file appendix_5_inf_alloc.tex]

\clearpage
\section*{GPU allocation algorithms}
\label{app:infer}

After building an ensemble, algorithms \ref{algo:alloc} and \ref{algo:speed} allows to deploy it efficiently on a GPU cluster.

\begin{algorithm}[h]
\caption{Allocate DNNs into GPUs cluster to fit into memory}
\label{algo:alloc}
\small
\begin{algorithmic}[1]

\STATE{\textbf{input:} $D$ the list of DNNs in the ensemble, $default\_batch\_size$, $ng$ the number of GPUs, $nc$ the number of CPUs}
\STATE{\textbf{output:} GPUs allocation $G$ and the CPUs allocation $C$. E.g. $G_{g}=[0,2]$ means that DNN 0 and DNN 2 are placed into the $g^{th}$ GPU}
\STATE{\textbf{start}}

\STATE{ // First structures are initialized}
\STATE{ $B_{i}$ $\gets$ $default\_batch\_size$, $i=0 ... length(D)$} 
\STATE{ $G_{g}$ $\gets$ [], $g=0 ... ng$ // for each GPU $g$ it associates its DNNs list}
\STATE{ $C_{c}$ $\gets$ [], $c=0 ... nc$}

\STATE{ $WG_{g}$ $\gets$ 0, $g=0 ... ng$  // for each GPU $g$ it associates its memory consumption} 
\STATE{ $WC_{c}$ $\gets$ 0, $c=0 ... nc$}
\STATE{ $I$ $\gets$ $fake\_images()$ // generate fake data to calibrate the allocation }

\STATE{ }
\STATE{ // Evaluation of the workload}
\STATE{ $DW$ $\gets$ [] }
\FOR{$i$ from 0 to length(D)}
\STATE{$DW$.append(nb\_weights($D[i]$))}
\ENDFOR
\STATE{ $D$ and $DW$ are sorted according $DW$ in desc. order}

\STATE{ }
\STATE{ // Allocation DNNs one by one from bigger to smaller DNN}
\STATE{ $current\_D$  $\gets$ [] }

\FOR{$i \gets 0$ to $length(D)$}
\STATE{ $current\_D$.append($D$[$i$])  }

\STATE{$gi$ $\gets$ $argmin(WG)$ //get the GPU with the least workload}
\STATE{$ci$ $\gets$ $argmin(WC)$ //get the CPU with the least workload}

\STATE{$G2$ $\gets$ $copy(G)$}
\STATE{$G2[gi]$.append($D$[$i$])}

\STATE{$C2$ $\gets$ $copy(C)$}
\STATE{$C2[ci]$.append($D$[$i$])}

// Where to place D[i] ?
\IF{bench($current\_D$,$B$,$G2$,$C$,$I$) $> 0$}
    \STATE{//D[i] is placed on GPU gi}
	\STATE{$G$ $\gets$ $G2$}
	\STATE{$WG$[$i$] $\gets$ $DW$[$i$] + $WG$[$i$]}
\ELSIF{bench($current\_D$,$B$,$G$,$C2$,$I$) $> 0$}
    \STATE{//D[i] is placed on CPU ci}
	\STATE{$C$ $\gets$ $C2$}
	\STATE{$WC$[$i$] $\gets$ $DW$[$i$] + $WC$[$i$]}
\ELSE
	\STATE{Error no device have enough memory}
\ENDIF

\ENDFOR
\STATE{return $\{G,C\}$}

\end{algorithmic}
\end{algorithm}

%%%%%%%%%%%%%%%%%%%%%%%%%%%%%%%%%%%%%%%%%

%%%%%%%%%%%%%%%%%%%%%%%%%%%%%%%%%%%%%%%%%%%%%%%%%%%%%%%%%%

\begin{algorithm}[]

\caption{Algorithm 2 - Refine GPUs allocation to speed up}
\label{algo:speed}
\begin{algorithmic}[1]

\STATE{\textbf{input:} $D$ the list of DNNs in the ensemble, $PB$ possible batch size values, $max_combi$ maximum number of assessed combinations, $G$ and $C$ are preliminary GPU and CPU allocation, $B$ preliminary batch sizes}
\STATE{\textbf{output:} $G$, $C$, $B$}
\STATE{\textbf{start}}

\STATE{ $I$ $\gets$ $fake\_images()$ // generate fake data to calibrate the allocation }

\STATE{ $current\_score$ $\gets$ bench($D$,$B$,$G$,$C$,$I$)}

\WHILE{$trials < max\_combi$}

\STATE{better\_allocs $\gets$ []}
\STATE{better\_scores $\gets$ []}

\STATE{$i\_allocs$  $\gets$ update\_i\_alloc($i$,$B$,$G$,$C$) }

\FORALL{$\{B2, G2, C2\}$ in $i\_allocs$}
\IF{$\{B, G, C\} \neq \{B2, G2, C2\}$}
\STATE{$score2$ $\gets$ bench($D$,$B2$,$G2$,$C2$,$I$)}
\IF{$score2 > current\_score$}
    \STATE{$better\_scores$.append($score2$)}
    \STATE{$better\_allocs$.append($\{B2, G2, C2\}$)}
\ENDIF
\IF{ $trials \geq max\_iter$ }
	\STATE{break}
\ENDIF

\ENDIF
\STATE{$trials \gets trials + 1$}

\ENDFOR

\IF{ length($better\_allocs$) > 0 }
    \STATE{$id$=argmax($better\_scores$)}
    \STATE{$\{B, G, C\}$ = $better\_scores$[$idbest$]}
    \STATE{$current\_score$=$better\_scores$[$idbest$]}
\ENDIF

\ENDWHILE

\STATE{return  $\{B, G, C\}$}

\end{algorithmic}

\end{algorithm}
