# Supplementary material for: A Deep Neural Networks ensemble workflow from hyperparameter search to inference leveraging GPU clusters
Source: arXiv:2208.14046 source file (2022-08-30)
Supplement: Supplementary file 5 [file appendix_4_resnet2.tex]

\clearpage
\section*{Replacing HPO by homogenous ResNet architectures}
\label{sec:res2}

% HPO > RESNET
We also compare our method with homogenous ensembling of ResNet architectures presented in figure~\ref{tab:appcompresfos}. For each architecture we repeat the training of models with the same computing effort i.e., 6 GPU during 6 days. Optimization settings are fixed, only the random seed diverse for each run time.

\begin{table}[h]
\centering
\small
\setlength\tabcolsep{2pt}
\begin{tabularx}{\linewidth}{lrrrrrr}
\toprule
\multicolumn{7}{c}{CIFAR100 dataset}\\
ResNet archi.  &    R18 & R34 & R50 & RX50 & R101 & R152   \\
\#weights of 1    & 31.6M & 53.1M & 53.1M & 13.1M & 95.8M    & 128.4M  \\
Cost & 10.83 & 14.35 & 14.05 & 11.87 & 21.14 & 28.56 \\
\midrule
\#1        & \textbf{35.30}                                                                                            & 35.77                                                                                           & 37.63                                                                                           & 42.28                                                                                            & 35.85                                                                                            & 37.82                                                                                             \\
\#2  & 32.98                                                                                            & \textbf{21.70}                                                                                           & 33.60                                                                                           & 38.67                                                                                            & 32.77                                                                                            & 34.86                                                                                             \\
\#3  & 29.88                                                                                            & \textbf{28.58}                                                                                           & 31.29                                                                                           & 36.16                                                                                            & 30.30                                                                                            & 32.16                                                                                             \\
\#4  & 28.66                                                                                            & \textbf{27.63}                                                                                           & 29.76                                                                                           & 35.09                                                                                            & 29.74                                                                                            & 31.65                                                                                             \\
\#6  & 27.70                                                                                            & \textbf{26.88}                                                                                           & 28.16                                                                                           & 32.15                                                                                            & 28.93                                                                                            & 30.26                                                                                             \\
\#8  & 26.98                                                                                            & \textbf{26.21}                                                                                           & 27.33                                                                                           & 31.86                                                                                            & 28.26                                                                                            & 29.33                                                                                             \\
\#12 & 26.59                                                                                            & \textbf{25.88}                                                                                           & 26.82                                                                                           & 31.44                                                                                            & 71.85                                                                                            & 29.46                                                                                             \\
\#16 & 26.66                                                                                            & \textbf{25.74}                                                                                           & 26.80                                                                                           & 31.44                                                                                            & 28.15                                                                                            & 29.45                                                                \\                            
\hline
\multicolumn{7}{c}{The microfossils dataset}\\
ResNet archi.  &    R18 & R34 & R50 & RX50 & R101 & R152   \\
\#weights of 1     & 31.6M & 53.1M & 53.1M & 13.1M & 95.8M    & 128.4M  \\
Cost     & 120.53 & 169.71 & 164.96 & 118.64 & 254.45    & 354.29  \\
\hline 
\#1 & \textbf{13.17}                                          & 14.76                                                  & 14.35                                                  & 15.09                                                   & 15.78                                                   & 14.91                                                    \\
\#2         & 12.26                                                   & \textbf{12.23}                                         & 12.46                                                  & 12.74                                                   & 13.96                                                   & 13.39                                                    \\

\#3         & 11.78                                                   & \textbf{11.45}                                         & 11.52                                                  & 12.07                                                   & 12.46                                                   & 12.34                                                    \\
\#4         & 11.66                                                   & \textbf{11.29}                                         & 11.37                                                  & 11.98                                                   & 12.26                                                   & 12.09                                                    \\
\#6         & 10.90                                                   & \textbf{10.50}                                         & 10.73                                                  & 11.73                                                   & 11.76                                                   & 11.32                                                    \\
\#8         & 10.87                                                   & \textbf{10.41}                                         & 10.61                                                  & 11.27                                                   & 11.60                                                   & 11.20 \\                                                   
\bottomrule
\end{tabularx}
\caption{Homogenous ensembling accuracy based on ResNet architectures. We vary the dataset, the ResNet architectures to build the library of models, and the ensemble size. We stop assessing to add models when it plateaus.}
\label{tab:appcompresfos}
\end{table}
