# Supplementary material for: A Deep Neural Networks ensemble workflow from hyperparameter search to inference leveraging GPU clusters
Source: arXiv:2208.14046 source file (2022-08-30)
Supplement: Supplementary file 6 [file appendix_6_combiner_rule.tex]

\clearpage
\section*{Combiner rule evaluation}
\label{app:combiner}

Table \ref{tab:combiner} and \ref{tab:combiner2} compare 6 ensemble with three different combiner rules. 

\begin{table}[h]
\centering
\small
\setlength\tabcolsep{3pt}
\begin{tabularx}{\linewidth}{l|cc|cc|cc}
\toprule
Budget             & \multicolumn{2}{c}{20}         & \multicolumn{2}{c}{80}         & \multicolumn{2}{c}{320}       \\
Metric        & Error            & CE              & Error            & CE              & Error            & CE              \\
\midrule
Maj. Voting        & \textbf{0.2643}          & 2.8047          & 0.2261          & 1.9208          & 0.2197          & 1.3622            \\
Averaging          & 0.278 & \textbf{1.1316} & 0.2202          & \textbf{0.8668} & \textbf{0.2042} & \textbf{0.7919}       \\
W. Averaging       & 0.2808          & 1.1362          & \textbf{0.2199} & 0.8691          & 0.2092          & 0.7921         \\
\bottomrule
\end{tabularx}

%\vspace{-0.2cm}
\caption{Forward greedy ensemble selection algorithm over the population of models trained with hyperband. We try three combiner rules: majority voting, averaging and weighted averaging.}
\label{tab:combiner}
\end{table}

\begin{table}[h]
\centering
\small
\setlength\tabcolsep{3pt}
\begin{tabularx}{\linewidth}{l|cc|cc|cc}
\toprule
Budget             & \multicolumn{2}{c}{20}         & \multicolumn{2}{c}{80}         & \multicolumn{2}{c}{320}         \\
Metric                        & Error            & CE              & Error            & CE              & Error            & CE              \\
\midrule
Maj. Voting           & 0.2663          & 2.5460          & 0.2381          & 1.6657          & 0.2314          & 1.1860         \\
Averaging          & \textbf{0.2444} & \textbf{0.9458} & 0.2265          & 0.8679          & 0.2206          & 0.8445          \\
W. Averaging        & 0.2450          & 0.9461          & \textbf{0.2258} & \textbf{0.8647} & \textbf{0.2204} & \textbf{0.8414} \\
\bottomrule
\end{tabularx}
%\vspace{-0.2cm}
\caption{Forward greed ensemble selection algorithm over the population of models trained with SMAC. We try three combiner rules: majority voting, averaging and weighted averaging.}
\label{tab:combiner2}
\end{table}
