# Supplementary material for: A Deep Neural Networks ensemble workflow from hyperparameter search to inference leveraging GPU clusters
Source: arXiv:2208.14046 source file (2022-08-30)
Supplement: Supplementary file 7 [file appendix_8_hpo.tex]

\clearpage
\section{HPO + Post-hoc ensembling with SMOBF}
\label{app:hpo}

Table \ref{tab:comphpocifar} and \ref{tab:comphpofos} is the evaluation of different workflow by varying the HPO algorithm to produce different libraries of models.

\begin{table}[]
\centering
\small
\setlength\tabcolsep{2pt}
\begin{tabularx}{8cm}{l|ccccccc}
\toprule
Budget    & RS             & HB             & BOGP  & BOHB           & SMAC           & TPE   & GA             \\
\midrule
20  & 31.26          & 27.8           & 31.58 & 29.24          & \textbf{24.44} & 29.97 & 24.61          \\
40  & 24.24          & \textbf{22.87}          & 28.2 & 25.6           & 22.97 & 26.01 & 22.91          \\
60  & 22.27          & 21.85          & 26.91 & 23.53          & 22.65          & 25.44 & \textbf{21.51} \\
80  & 22.69          & 21.73          & 26.2  & 22.58          & 22.17          & 24.25 &  \textbf{21.07} \\
120 & 21.63          & \textbf{21.55}          & 24.78 & 21.86 & 22.17          & 23.03 & 21.95          \\
160 & \textbf{20.11} & \textbf{21.11} & 24.24 & 21.64          & 21.87          & 22.47 & 21.91          \\
240 & 20.7           & \textbf{20.46}          & 23.76 & 21.2           & 21.87          & 22.55 & 21.91          \\
320 & 20.64          & \textbf{20.42} & 23.76 & 21.1           & 21.87          & 22.46 & 21.91         \\
\bottomrule
\end{tabularx}
\caption{Our AutoML by comparing seven HPO algorithms was run on CIFAR100 during 6 days on 6 GPUs generating seven libraries of models. Numbers are expressed in percentage error.}
\label{tab:comphpocifar}
\end{table}

\begin{table}[]
\centering
\small
\setlength\tabcolsep{3pt}
\begin{tabularx}{\columnwidth}{l|rrrrrrr}
\toprule
Budget     & RS    & HB            & BOGP  & BOHB  & SMAC           & TPE   & GA    \\
\midrule
125  & 13.45 & 11.93         & 14.44 & 12.18 & \textbf{10.27} & 13.91 & 10.33 \\
250  & 10.98 & 9.82          & 10.93 & 11.71 & \textbf{9.63}  & 10.66 & 9.71  \\
375  & 10.84 & \textbf{9.32} & 9.93  & 10.5  & 9.45           & 10.49 & 9.5   \\
500  & 10.23 & \textbf{8.91} & 9.93  & 9.84  & 9.27           & 9.06  & 9.28  \\
750 & 9.7   & \textbf{8.87} & 9.21  & 9.28  & 9.18           & 9.3   & 9.18  \\
1000 & 9.69  & \textbf{8.46} & 8.77  & 8.8   & 9.09           & 9.21  & 9.07 \\
\bottomrule
\end{tabularx}
\caption{Our AutoML by comparing seven HPO algorithms was run on the microfossils dataset during 6 days on 6 GPUs generating seven libraries of models.}
\label{tab:comphpofos}
\end{table}
