# Supplementary material for: A Deep Neural Networks ensemble workflow from hyperparameter search to inference leveraging GPU clusters
Source: arXiv:2208.14046 source file (2022-08-30)
Supplement: Supplementary file 8 [file appendix_hpo_scal.tex]

\section*{Scalability of HPO algorithms}

% Benchmarking is challenging
Our CNN framework based on ResNet can takes between 15 seconds and 11min30 regarding the complexity of the neural architecture assessed. 

\begin{table*}[]
\begin{tabularx}{\linewidth}{l|lllll|lllll}
\toprule
                & \multicolumn{5}{c}{9 trials 100 epochs}                                     & \multicolumn{5}{c}{30   trials 30 epochs}                                   \\
                & acc (\%)                        & duration & speed up & \#epochs & gpu (\%) & acc (\%)                        & duration & speed up & \#epochs & gpu (\%) \\
\midrule
RS 6GPUs        & $67.08\pm3.85$                  & 10h13    & 6.2      & 900      & 85       & 64.90+-0.92                     & 11h40    & 5.5      & 900      & 82       \\
\hline
HB 6GPUs        & \multirow{2}{*}{$62.58\pm4.73$} & 5h48     & 4.4      & 710      & 49       & \multirow{2}{*}{$62.94\pm5.28$} & 1h40     & 5.2      & 388      & 62       \\
HB 4nodes*6GPUs &                                 & 2h00     & 8.8      & 710      & 33       &                                 & 0h48     & 10.9     & 388      & 34       \\
\hline
GA 6GPUs        & $61.85\pm2.55$                  & 14h29    & 2.8      & 900      & 27       & $65.33\pm2.33$                  & 10h01    & 4.1      & 900      & 57      \\
\bottomrule
\end{tabularx}
\caption{Limited scale benchmarks of some HPO algorithms. Hyperband was set up with a halving of 3 and the genetic the number of trials is divided into 3 successive generations. The columns from the left to the right are: The accuracy error which is not dependant of the number of resources, the duration of the HPO process, the speed up measured compared to the single GPU version, the  \#epochs is the number of train iteration performed, the mean percentage of occupied GPU during all the entire HPO process.}
\label{tab:bench}
\end{table*}

% Hyperband avantage
Despite those challenges, our benchmark reveal that Random Search and Hyperband leave less GPUs vacant than GA which is explained by the fact that no intermediate stopping of all GPUs is required. Those benchmarks also confirm that Hyperband terminates earlier than Random Search because the less promising DNNs have been stopped before the maximum number of epochs. The scalability and saving useless computations are two important algorithmic characteristics for speed up this type of application.

% Termination
At the end of any algorithm the last DNNs free the GPUs but they take various amount of time to terminate, this is explained why we measure not a perfect usage of GPUs of Random Search and Hyperband. Furthermore, Hyperband emphasis this phenomenon because the early stopping increases the variability of time took between DNNs.
